# Supplementary material for: Program Structure Aware Precondition Generation
Source: arXiv:2310.02154 source file (2024-08-16)
Supplement: Supplementary file 1 [file 9_appendix_full.tex]

\pagebreak
\section{Appendix}
\label{sec:app}

\subsection{User Study Samples}

%
% PRECONDITION 1
%

\begin{figure}
    \begin{subfigure}{\linewidth}
    \centering
    \lstset{style=mystyle, xleftmargin=.0\textwidth, xrightmargin=0.\textwidth, linewidth=0.0\linewidth}
    \lstinputlisting[linewidth=4.8cm]{./user_study/P1/input1.java}
    \label{fig:p1:i1}
    \end{subfigure}
    
    \begin{subfigure}[p]{\linewidth}
    \lstset{style=mystyle, xleftmargin=.0\textwidth, xrightmargin=0.\textwidth, linewidth=0.0\linewidth}
    \lstinputlisting[linewidth=4.8cm]{./examples/DivideAndRemainder/DivideAndRemainder_mine.java}
    \label{fig:p1:ours}
    \end{subfigure}
  \caption{Precondition 1, Input 1, Group A.}
  \label{fig:P2}
\end{figure}
\begin{figure}
    \begin{subfigure}{\linewidth}
    \centering
    \lstset{style=mystyle, xleftmargin=.0\textwidth, xrightmargin=0.\textwidth, linewidth=0.0\linewidth}
    \lstinputlisting[linewidth=4.8cm]{./user_study/P1/input2.java}
    \label{fig:p1:i1}
    \end{subfigure}
    
    \begin{subfigure}[p]{\linewidth}
    \lstset{style=mystyle, xleftmargin=.0\textwidth, xrightmargin=0.\textwidth, linewidth=0.0\linewidth}
    \lstinputlisting[linewidth=4.8cm]{./examples/DivideAndRemainder/DivideAndRemainder_mine.java}
    \label{fig:p1:ours}
    \end{subfigure}
    
  \caption{Precondition 1, Input 2, Group A.}
  \label{fig:P2}
\end{figure}
\begin{figure}
    \begin{subfigure}{\linewidth}
    \centering
    \lstset{style=mystyle, xleftmargin=.0\textwidth, xrightmargin=0.\textwidth, linewidth=0.0\linewidth}
    \lstinputlisting[linewidth=4.8cm]{./user_study/P1/input3.java}
    \label{fig:p1:i1}
    \end{subfigure}
    
    \begin{subfigure}[p]{\linewidth}
    \lstset{style=mystyle, xleftmargin=.0\textwidth, xrightmargin=0.\textwidth, linewidth=0.0\linewidth}
    \lstinputlisting[linewidth=4.8cm]{./examples/DivideAndRemainder/DivideAndRemainder_mine.java}
    \label{fig:p1:ours}
    \end{subfigure}
    
  \caption{Precondition 1, Input 3, Group A.}
  \label{fig:P2}
\end{figure}

%
%  PRECONDITION 1, GROUP B
%

\begin{figure}
    \begin{minipage}{.4\linewidth}

    \begin{subfigure}{\linewidth}
        \lstset{style=mystyle, xleftmargin=.0\textwidth, xrightmargin=0.\textwidth, linewidth=0.0\linewidth}
    \lstinputlisting[linewidth=6cm]{./user_study/P1/input1.java}
    \label{fig:p1:i1}
    %\vspace{-0.15in}
    \end{subfigure}
    \begin{subfigure}[p]{\linewidth}
    \centering

    \lstset{style=mystyle, xleftmargin=.0\textwidth, xrightmargin=0.0\textwidth, linewidth=0.0\linewidth}
    \lstinputlisting[linewidth=6cm]{./examples/DivideAndRemainder/DivideAndRemainder_theirs_us.java}
    \label{fig:p1:ours}
    \end{subfigure}
    \end{minipage}
    \hfill
    \begin{minipage}{.54\linewidth}
    \vspace{1.2cm}
    \begin{subfigure}[p]{\linewidth}
    \lstset{style=mystyle, xleftmargin=.0\textwidth, xrightmargin=0.\textwidth, linewidth=0.0\linewidth}
    \lstinputlisting[linewidth=7cm]{./examples/DivideAndRemainder/context_theirs.java}
    \label{fig:p1:ours}
    \end{subfigure}
        \end{minipage}

  \caption{Precondition 1, Input 1, Group B.}
  \label{fig:P2}
\end{figure}
\begin{figure}
    \begin{minipage}{.4\linewidth}

    \begin{subfigure}{\linewidth}
        \lstset{style=mystyle, xleftmargin=.0\textwidth, xrightmargin=0.\textwidth, linewidth=0.0\linewidth}
    \lstinputlisting[linewidth=6cm]{./user_study/P1/input2.java}
    \label{fig:p1:i1}
    %\vspace{-0.15in}
    \end{subfigure}
    \begin{subfigure}[p]{\linewidth}
    \centering

    \lstset{style=mystyle, xleftmargin=.0\textwidth, xrightmargin=0.0\textwidth, linewidth=0.0\linewidth}
    \lstinputlisting[linewidth=6cm]{./examples/DivideAndRemainder/DivideAndRemainder_theirs_us.java}
    \label{fig:p1:ours}
    \end{subfigure}
    \end{minipage}
    \hfill
    \begin{minipage}{.54\linewidth}
    \vspace{2.2cm}
    \begin{subfigure}[p]{\linewidth}
    \lstset{style=mystyle, xleftmargin=.0\textwidth, xrightmargin=0.\textwidth, linewidth=0.0\linewidth}
    \lstinputlisting[linewidth=7cm]{./examples/DivideAndRemainder/context_theirs.java}
    \label{fig:p1:ours}
    \end{subfigure}
        \end{minipage}

  \caption{Precondition 1, Input 2, Group B.}
  \label{fig:P2}
\end{figure}
\begin{figure}
    \begin{minipage}{.4\linewidth}

    \begin{subfigure}{\linewidth}
        \lstset{style=mystyle, xleftmargin=.0\textwidth, xrightmargin=0.\textwidth, linewidth=0.0\linewidth}
    \lstinputlisting[linewidth=6cm]{./user_study/P1/input3.java}
    \label{fig:p1:i1}
    %\vspace{-0.15in}
    \end{subfigure}
    \begin{subfigure}[p]{\linewidth}
    \centering

    \lstset{style=mystyle, xleftmargin=.0\textwidth, xrightmargin=0.0\textwidth, linewidth=0.0\linewidth}
    \lstinputlisting[linewidth=6cm]{./examples/DivideAndRemainder/DivideAndRemainder_theirs_us.java}
    \label{fig:p1:ours}
    \end{subfigure}
    \end{minipage}
    \hfill
    \begin{minipage}{.54\linewidth}
    \vspace{2.2cm}
    \begin{subfigure}[p]{\linewidth}
    \lstset{style=mystyle, xleftmargin=.0\textwidth, xrightmargin=0.\textwidth, linewidth=0.0\linewidth}
    \lstinputlisting[linewidth=7cm]{./examples/DivideAndRemainder/context_theirs.java}
    \label{fig:p1:ours}
    \end{subfigure}
        \end{minipage}

  \caption{Precondition 1, Input 3, Group B.}
  \label{fig:P2}
\end{figure}

\pagebreak

%
% PRECONDITION 2
%

\begin{figure}
    \begin{minipage}{.4\linewidth}
    \begin{subfigure}{\linewidth}
    \centering

    \lstset{style=mystyle, xleftmargin=.0\textwidth, xrightmargin=0.0\textwidth, linewidth=0.0\linewidth}
    \lstinputlisting[linewidth=13.4cm]{./user_study/P2/input1.java}
    %\hspace{.3cm}\includegraphics[width=5cm]{./user_study/P2/input1.png}
    \label{fig:p1:i1}
    %\vspace{-0.15in}
    \end{subfigure}
    \begin{subfigure}[p]{\linewidth}
    \centering

    \lstset{style=mystyle, xleftmargin=.0\textwidth, xrightmargin=0.0\textwidth, linewidth=0.0\linewidth}
    \lstinputlisting[linewidth=6cm]{./examples/Max/Max_ours.java}
    \label{fig:p1:ours}
    \end{subfigure}
    \end{minipage}
    \hfill
    \begin{minipage}{.54\linewidth}
    \vspace{2.2cm}
    \begin{subfigure}[p]{\linewidth}
    \lstset{style=mystyle, xleftmargin=.0\textwidth, xrightmargin=0.\textwidth, linewidth=0.0\linewidth}
    \lstinputlisting[linewidth=7cm]{./examples/Max/Max_context.java}
    \label{fig:p1:ours}
    \end{subfigure}
    \end{minipage}

  \caption{Precondition 2, Input 1, Group A.}
  \label{fig:P2}
\end{figure}
\begin{figure}
    \begin{minipage}{.4\linewidth}
    \begin{subfigure}{\linewidth}
    \centering

    \lstset{style=mystyle, xleftmargin=.0\textwidth, xrightmargin=0.0\textwidth, linewidth=0.0\linewidth}
    \lstinputlisting[linewidth=13.4cm]{./user_study/P2/input2.java}
    %\hspace{.3cm}\includegraphics[width=5cm]{./user_study/P2/input1.png}
    \label{fig:p1:i1}
    %\vspace{-0.15in}
    \end{subfigure}
    \begin{subfigure}[p]{\linewidth}
    \centering

    \lstset{style=mystyle, xleftmargin=.0\textwidth, xrightmargin=0.0\textwidth, linewidth=0.0\linewidth}
    \lstinputlisting[linewidth=6cm]{./examples/Max/Max_ours.java}
    \label{fig:p1:ours}
    \end{subfigure}
    \end{minipage}
    \hfill
    \begin{minipage}{.54\linewidth}
    \vspace{2.2cm}
    \begin{subfigure}[p]{\linewidth}
    \lstset{style=mystyle, xleftmargin=.0\textwidth, xrightmargin=0.\textwidth, linewidth=0.0\linewidth}
    \lstinputlisting[linewidth=7cm]{./examples/Max/Max_context.java}
    \label{fig:p1:ours}
    \end{subfigure}
    \end{minipage}

  \caption{Precondition 2, Input 2, Group A.}
  \label{fig:P2}
\end{figure}
\begin{figure}
    \begin{minipage}{.4\linewidth}
    \begin{subfigure}{\linewidth}
    \centering

    \lstset{style=mystyle, xleftmargin=.0\textwidth, xrightmargin=0.0\textwidth, linewidth=0.0\linewidth}
    \lstinputlisting[linewidth=13.4cm]{./user_study/P2/input3.java}
    %\hspace{.3cm}\includegraphics[width=5cm]{./user_study/P2/input1.png}
    \label{fig:p1:i1}
    %\vspace{-0.15in}
    \end{subfigure}
    \begin{subfigure}[p]{\linewidth}
    \centering

    \lstset{style=mystyle, xleftmargin=.0\textwidth, xrightmargin=0.0\textwidth, linewidth=0.0\linewidth}
    \lstinputlisting[linewidth=6cm]{./examples/Max/Max_ours.java}
    \label{fig:p1:ours}
    \end{subfigure}
    \end{minipage}
    \hfill
    \begin{minipage}{.54\linewidth}
    \vspace{2.2cm}
    \begin{subfigure}[p]{\linewidth}
    \lstset{style=mystyle, xleftmargin=.0\textwidth, xrightmargin=0.\textwidth, linewidth=0.0\linewidth}
    \lstinputlisting[linewidth=7cm]{./examples/Max/Max_context.java}
    \label{fig:p1:ours}
    \end{subfigure}
    \end{minipage}

  \caption{Precondition 2, Input 3, Group A.}
  \label{fig:P2}
\end{figure}

% GROUP B

\begin{figure}
    \begin{subfigure}{\linewidth}
    \centering
    \lstset{style=mystyle, xleftmargin=.0\textwidth, xrightmargin=0.\textwidth, linewidth=0.0\linewidth}
    \lstinputlisting[linewidth=6cm]{./user_study/P2/input1_nc.java}
    \label{fig:p1:i1}
    \end{subfigure}
    
    \begin{subfigure}[p]{\linewidth}
    \lstset{style=mystyle, xleftmargin=.0\textwidth, xrightmargin=0.\textwidth, linewidth=0.0\linewidth}
    \lstinputlisting[linewidth=6cm]{./examples/Max/Max_theirs.java}

    \label{fig:p1:ours}
    \end{subfigure}
    
  \caption{Precondition 2, Input 1, Group B.}
  \label{fig:P2}
\end{figure}
\begin{figure}
    \begin{subfigure}{\linewidth}
    \centering
    \lstset{style=mystyle, xleftmargin=.0\textwidth, xrightmargin=0.\textwidth, linewidth=0.0\linewidth}
    \lstinputlisting[linewidth=6cm]{./user_study/P2/input2_nc.java}
    \label{fig:p1:i1}
    \end{subfigure}
    
    \begin{subfigure}[p]{\linewidth}
    \lstset{style=mystyle, xleftmargin=.0\textwidth, xrightmargin=0.\textwidth, linewidth=0.0\linewidth}
    \lstinputlisting[linewidth=6cm]{./examples/Max/Max_theirs.java}
    \label{fig:p1:ours}
    \end{subfigure}
    
  \caption{Precondition 2, Input 2, Group B.}
  \label{fig:P2}
\end{figure}
\begin{figure}
    \begin{subfigure}{\linewidth}
    \centering
    \lstset{style=mystyle, xleftmargin=.0\textwidth, xrightmargin=0.\textwidth, linewidth=0.0\linewidth}
    \lstinputlisting[linewidth=6cm]{./user_study/P2/input3_nc.java}
    \label{fig:p1:i1}
    \end{subfigure}
    
    \begin{subfigure}[p]{\linewidth}
    \lstset{style=mystyle, xleftmargin=.0\textwidth, xrightmargin=0.\textwidth, linewidth=0.0\linewidth}
    \lstinputlisting[linewidth=6cm]{./examples/Max/Max_theirs.java}
    \label{fig:p1:ours}
    \end{subfigure}
    
  \caption{Precondition 2, Input 3, Group B.}
  \label{fig:P2}
\end{figure}

%
% PRECONDITION 3
%

\begin{figure}
    \begin{subfigure}{\linewidth}
    \centering
    \lstset{style=mystyle, xleftmargin=.0\textwidth, xrightmargin=0.\textwidth, linewidth=0.0\linewidth}
    \lstinputlisting[linewidth=11cm]{./user_study/P3/input1.java}
    \label{fig:p1:i1}
    \end{subfigure}
    
    \begin{subfigure}[p]{\linewidth}
    \lstset{style=mystyle, xleftmargin=.0\textwidth, xrightmargin=0.\textwidth, linewidth=0.0\linewidth}
    \lstinputlisting[linewidth=11cm]{./examples/Add/Add_ours.java}

    \label{fig:p1:ours}
    \end{subfigure}
    
  \caption{Precondition 3, Input 1, Group A.}
  \label{fig:P2}
\end{figure}
\begin{figure}
    \begin{subfigure}{\linewidth}
    \centering
    \lstset{style=mystyle, xleftmargin=.0\textwidth, xrightmargin=0.\textwidth, linewidth=0.0\linewidth}
    \lstinputlisting[linewidth=11cm]{./user_study/P3/input2.java}
    \label{fig:p1:i1}
    \end{subfigure}

    \begin{subfigure}[p]{\linewidth}
    \lstset{style=mystyle, xleftmargin=.0\textwidth, xrightmargin=0.\textwidth, linewidth=0.0\linewidth}
    \lstinputlisting[linewidth=11cm]{./examples/Add/Add_ours.java}
    \label{fig:p1:ours}
    \end{subfigure}
    
  \caption{Precondition 3, Input 2, Group A.}
  \label{fig:P2}
\end{figure}
\begin{figure}
    \begin{subfigure}{\linewidth}
    \centering
    \lstset{style=mystyle, xleftmargin=.0\textwidth, xrightmargin=0.\textwidth, linewidth=0.0\linewidth}
    \lstinputlisting[linewidth=11cm]{./user_study/P3/input3.java}
    \label{fig:p1:i1}
    \end{subfigure}
    
    \begin{subfigure}[p]{\linewidth}
    \lstset{style=mystyle, xleftmargin=.0\textwidth, xrightmargin=0.\textwidth, linewidth=0.0\linewidth}
    \lstinputlisting[linewidth=11cm]{./examples/Add/Add_ours.java}
    \label{fig:p1:ours}
    \end{subfigure}
    
  \caption{Precondition 3, Input 3, Group A.}
  \label{fig:P2}
\end{figure}

% GROUP B

\begin{figure}
    \begin{minipage}{.4\linewidth}
    \begin{subfigure}{\linewidth}
    \centering

    \lstset{style=mystyle, xleftmargin=.0\textwidth, xrightmargin=0.0\textwidth, linewidth=0.0\linewidth}
    \lstinputlisting[linewidth=13.4cm]{./user_study/P3/input1.java}
    %\hspace{.3cm}\includegraphics[width=5cm]{./user_study/P2/input1.png}
    \label{fig:p1:i1}
    %\vspace{-0.15in}
    \end{subfigure}
    \begin{subfigure}[p]{\linewidth}
    \centering

    \lstset{style=mystyle, xleftmargin=.0\textwidth, xrightmargin=0.0\textwidth, linewidth=0.0\linewidth}
    \lstinputlisting[linewidth=6cm]{./examples/Add/Add_theirs.java}
    \label{fig:p1:ours}
    \end{subfigure}
    \end{minipage}
    \hfill
    \begin{minipage}{.54\linewidth}
    \vspace{2.2cm}
    \begin{subfigure}[p]{\linewidth}
    \lstset{style=mystyle, xleftmargin=.0\textwidth, xrightmargin=0.\textwidth, linewidth=0.0\linewidth}
    \lstinputlisting[linewidth=7cm]{./examples/Add/Add_context.java}
    \label{fig:p1:ours}
    \end{subfigure}
    \end{minipage}

  \caption{Precondition 3, Input 1, Group B.}
  \label{fig:P2}
\end{figure}
\begin{figure}
    \begin{minipage}{.4\linewidth}
    \begin{subfigure}{\linewidth}
    \centering

    \lstset{style=mystyle, xleftmargin=.0\textwidth, xrightmargin=0.0\textwidth, linewidth=0.0\linewidth}
    \lstinputlisting[linewidth=13.4cm]{./user_study/P3/input2.java}
    %\hspace{.3cm}\includegraphics[width=5cm]{./user_study/P2/input1.png}
    \label{fig:p1:i1}
    %\vspace{-0.15in}
    \end{subfigure}
    \begin{subfigure}[p]{\linewidth}
    \centering

    \lstset{style=mystyle, xleftmargin=.0\textwidth, xrightmargin=0.0\textwidth, linewidth=0.0\linewidth}
    \lstinputlisting[linewidth=6cm]{./examples/Add/Add_theirs.java}
    \label{fig:p1:ours}
    \end{subfigure}
    \end{minipage}
    \hfill
    \begin{minipage}{.54\linewidth}
    \vspace{2.2cm}
    \begin{subfigure}[p]{\linewidth}
    \lstset{style=mystyle, xleftmargin=.0\textwidth, xrightmargin=0.\textwidth, linewidth=0.0\linewidth}
    \lstinputlisting[linewidth=7cm]{./examples/Add/Add_context.java}
    \label{fig:p1:ours}
    \end{subfigure}
    \end{minipage}

  \caption{Precondition 3, Input 2, Group B.}
  \label{fig:P2}
\end{figure}
\begin{figure}
    \begin{minipage}{.4\linewidth}
    \begin{subfigure}{\linewidth}
    \centering

    \lstset{style=mystyle, xleftmargin=.0\textwidth, xrightmargin=0.0\textwidth, linewidth=0.0\linewidth}
    \lstinputlisting[linewidth=13.4cm]{./user_study/P3/input3.java}
    %\hspace{.3cm}\includegraphics[width=5cm]{./user_study/P2/input1.png}
    \label{fig:p1:i1}
    %\vspace{-0.15in}
    \end{subfigure}
    \begin{subfigure}[p]{\linewidth}
    \centering

    \lstset{style=mystyle, xleftmargin=.0\textwidth, xrightmargin=0.0\textwidth, linewidth=0.0\linewidth}
    \lstinputlisting[linewidth=6cm]{./examples/Add/Add_theirs.java}
    \label{fig:p1:ours}
    \end{subfigure}
    \end{minipage}
    \hfill
    \begin{minipage}{.54\linewidth}
    \vspace{2.2cm}
    \begin{subfigure}[p]{\linewidth}
    \lstset{style=mystyle, xleftmargin=.0\textwidth, xrightmargin=0.\textwidth, linewidth=0.0\linewidth}
    \lstinputlisting[linewidth=7cm]{./examples/Add/Add_context.java}
    \label{fig:p1:ours}
    \end{subfigure}
    \end{minipage}

  \caption{Precondition 3, Input 3, Group B.}
  \label{fig:P2}
\end{figure}

%
% PRECONDITION 4
%

\begin{figure}
    \begin{subfigure}{\linewidth}
    \centering
    \lstset{style=mystyle, xleftmargin=.0\textwidth, xrightmargin=0.\textwidth, linewidth=0.0\linewidth}
    \lstinputlisting[linewidth=4.8cm]{./user_study/P4/input1.java}
    \label{fig:p1:i1}
    \end{subfigure}
    
    \begin{subfigure}[p]{\linewidth}
    \lstset{style=mystyle, xleftmargin=.0\textwidth, xrightmargin=0.\textwidth, linewidth=0.0\linewidth}
    \lstinputlisting[linewidth=4.8cm]{./examples/Mod/Mod_ours.java}
    \label{fig:p1:ours}
    \end{subfigure}
    
  \caption{Precondition 4, Input 1, Group A.}
  \label{fig:P2}
\end{figure}
\begin{figure}
    \begin{subfigure}{\linewidth}
    \centering
    \lstset{style=mystyle, xleftmargin=.0\textwidth, xrightmargin=0.\textwidth, linewidth=0.0\linewidth}
    \lstinputlisting[linewidth=4.8cm]{./user_study/P4/input2.java}
    \label{fig:p1:i1}
    \end{subfigure}
    
    \begin{subfigure}[p]{\linewidth}
    \lstset{style=mystyle, xleftmargin=.0\textwidth, xrightmargin=0.\textwidth, linewidth=0.0\linewidth}
    \lstinputlisting[linewidth=4.8cm]{./examples/Mod/Mod_ours.java}
    \label{fig:p1:ours}
    \end{subfigure}
    
  \caption{Precondition 4, Input 2, Group A.}
  \label{fig:P2}
\end{figure}
\begin{figure}
    \begin{subfigure}{\linewidth}
    \centering
    \lstset{style=mystyle, xleftmargin=.0\textwidth, xrightmargin=0.\textwidth, linewidth=0.0\linewidth}
    \lstinputlisting[linewidth=4.8cm]{./user_study/P4/input3.java}
    \label{fig:p1:i1}
    \end{subfigure}
    
    \begin{subfigure}[p]{\linewidth}
    \lstset{style=mystyle, xleftmargin=.0\textwidth, xrightmargin=0.\textwidth, linewidth=0.0\linewidth}
    \lstinputlisting[linewidth=4.8cm]{./examples/Mod/Mod_ours.java}
    \label{fig:p1:ours}
    \end{subfigure}
    
  \caption{Precondition 4, Input 3, Group A.}
  \label{fig:P2}
\end{figure}

% GROUP B

\begin{figure}
    \begin{subfigure}{\linewidth}
    \centering
    \lstset{style=mystyle, xleftmargin=.0\textwidth, xrightmargin=0.\textwidth, linewidth=0.0\linewidth}
    \lstinputlisting[linewidth=5.3cm]{./user_study/P4/input1.java}
    \label{fig:p1:i1}
    \end{subfigure}
    
    \begin{subfigure}[p]{\linewidth}
    \lstset{style=mystyle, xleftmargin=.0\textwidth, xrightmargin=0.\textwidth, linewidth=0.0\linewidth}
    \lstinputlisting[linewidth=5.3cm]{./examples/Mod/Mod_theirs.java}
    \label{fig:p1:ours}
    \end{subfigure}
    
  \caption{Precondition 4, Input 1, Group B.}
  \label{fig:P2}
\end{figure}
\begin{figure}
    \begin{subfigure}{\linewidth}
    \centering
    \lstset{style=mystyle, xleftmargin=.0\textwidth, xrightmargin=0.\textwidth, linewidth=0.0\linewidth}
    \lstinputlisting[linewidth=5.3cm]{./user_study/P4/input2.java}
    \label{fig:p1:i1}
    \end{subfigure}
    
    \begin{subfigure}[p]{\linewidth}
    \lstset{style=mystyle, xleftmargin=.0\textwidth, xrightmargin=0.\textwidth, linewidth=0.0\linewidth}
    \lstinputlisting[linewidth=5.3cm]{./examples/Mod/Mod_theirs.java}
    \label{fig:p1:ours}
    \end{subfigure}
    
  \caption{Precondition 4, Input 2, Group B.}
  \label{fig:P2}
\end{figure}
\begin{figure}
    \begin{subfigure}{\linewidth}
    \centering
    \lstset{style=mystyle, xleftmargin=.0\textwidth, xrightmargin=0.\textwidth, linewidth=0.0\linewidth}
    \lstinputlisting[linewidth=5.3cm]{./user_study/P4/input3.java}
    \label{fig:p1:i1}
    \end{subfigure}
    
    \begin{subfigure}[p]{\linewidth}
    \lstset{style=mystyle, xleftmargin=.0\textwidth, xrightmargin=0.\textwidth, linewidth=0.0\linewidth}
    \lstinputlisting[linewidth=5.3cm]{./examples/Mod/Mod_theirs.java}
    \label{fig:p1:ours}
    \end{subfigure}
    
  \caption{Precondition 4, Input 3, Group B.}
  \label{fig:P2}
\end{figure}

%
%   PRECONDITION 5
%

\begin{figure}
    \begin{minipage}{.4\linewidth}
    \begin{subfigure}{\linewidth}
    \centering

    \lstset{style=mystyle, xleftmargin=.0\textwidth, xrightmargin=0.0\textwidth, linewidth=0.0\linewidth}
    \lstinputlisting[linewidth=14cm]{./user_study/P5/input1.java}
    %\hspace{.3cm}\includegraphics[width=5cm]{./user_study/P2/input1.png}
    \label{fig:p1:i1}
    %\vspace{-0.15in}
    \end{subfigure}
    \begin{subfigure}[p]{\linewidth}
    \centering

    \lstset{style=mystyle, xleftmargin=.0\textwidth, xrightmargin=0.0\textwidth, linewidth=0.0\linewidth}
    \lstinputlisting[linewidth=6cm]{./examples/GCD/GCD_ours.java}
    \label{fig:p1:ours}
    \end{subfigure}
    \end{minipage}
    \hfill
    \begin{minipage}{.54\linewidth}
    \vspace{2.2cm}
    \begin{subfigure}[p]{\linewidth}
    \lstset{style=mystyle, xleftmargin=.0\textwidth, xrightmargin=0.\textwidth, linewidth=0.0\linewidth}
    \lstinputlisting[linewidth=7.6cm]{./examples/GCD/GCD_context1_ours.java}
    \label{fig:p1:ours}
    \end{subfigure}
    \end{minipage}

  \caption{Precondition 5, Input 1, Group A.}
  \label{fig:P2}
\end{figure}
\begin{figure}
    \begin{minipage}{.4\linewidth}
    \begin{subfigure}{\linewidth}
    \centering

    \lstset{style=mystyle, xleftmargin=.0\textwidth, xrightmargin=0.0\textwidth, linewidth=0.0\linewidth}
    \lstinputlisting[linewidth=14cm]{./user_study/P5/input2.java}
    %\hspace{.3cm}\includegraphics[width=5cm]{./user_study/P2/input1.png}
    \label{fig:p1:i1}
    %\vspace{-0.15in}
    \end{subfigure}
    \begin{subfigure}[p]{\linewidth}
    \centering

    \lstset{style=mystyle, xleftmargin=.0\textwidth, xrightmargin=0.0\textwidth, linewidth=0.0\linewidth}
    \lstinputlisting[linewidth=6cm]{./examples/GCD/GCD_ours.java}
    \label{fig:p1:ours}
    \end{subfigure}
    \end{minipage}
    \hfill
    \begin{minipage}{.54\linewidth}
    \vspace{2.2cm}
    \begin{subfigure}[p]{\linewidth}
    \lstset{style=mystyle, xleftmargin=.0\textwidth, xrightmargin=0.\textwidth, linewidth=0.0\linewidth}
    \lstinputlisting[linewidth=7.6cm]{./examples/GCD/GCD_context1_ours.java}
    \label{fig:p1:ours}
    \end{subfigure}
    \end{minipage}

  \caption{Precondition 5, Input 2, Group A.}
  \label{fig:P2}
\end{figure}
\begin{figure}
    \begin{minipage}{.4\linewidth}
    \begin{subfigure}{\linewidth}
    \centering

    \lstset{style=mystyle, xleftmargin=.0\textwidth, xrightmargin=0.0\textwidth, linewidth=0.0\linewidth}
    \lstinputlisting[linewidth=14cm]{./user_study/P5/input3.java}
    %\hspace{.3cm}\includegraphics[width=5cm]{./user_study/P2/input1.png}
    \label{fig:p1:i1}
    %\vspace{-0.15in}
    \end{subfigure}
    \begin{subfigure}[p]{\linewidth}
    \centering

    \lstset{style=mystyle, xleftmargin=.0\textwidth, xrightmargin=0.0\textwidth, linewidth=0.0\linewidth}
    \lstinputlisting[linewidth=6cm]{./examples/GCD/GCD_ours.java}
    \label{fig:p1:ours}
    \end{subfigure}
    \end{minipage}
    \hfill
    \begin{minipage}{.54\linewidth}
    \vspace{2.2cm}
    \begin{subfigure}[p]{\linewidth}
    \lstset{style=mystyle, xleftmargin=.0\textwidth, xrightmargin=0.\textwidth, linewidth=0.0\linewidth}
    \lstinputlisting[linewidth=7.6cm]{./examples/GCD/GCD_context1_ours.java}
    \label{fig:p1:ours}
    \end{subfigure}
    \end{minipage}

  \caption{Precondition 5, Input 3, Group A.}
  \label{fig:P2}
\end{figure}

% GROUP B

\begin{figure}
    \begin{subfigure}{\linewidth}
    \centering
    \lstset{style=mystyle, xleftmargin=.0\textwidth, xrightmargin=0.\textwidth, linewidth=0.0\linewidth}
    \lstinputlisting[linewidth=8cm]{./user_study/P5/input1.java}
    \label{fig:p1:i1}
    \end{subfigure}
    
    \begin{subfigure}[p]{\linewidth}
    \lstset{style=mystyle, xleftmargin=.0\textwidth, xrightmargin=0.\textwidth, linewidth=0.0\linewidth}
    \lstinputlisting[linewidth=8cm]{./examples/GCD/GCD_theirs.java}
    \label{fig:p1:ours}
    \end{subfigure}
    
  \caption{Precondition 5, Input 1, Group B.}
  \label{fig:P2}
\end{figure}
\begin{figure}
    \begin{subfigure}{\linewidth}
    \centering
    \lstset{style=mystyle, xleftmargin=.0\textwidth, xrightmargin=0.\textwidth, linewidth=0.0\linewidth}
    \lstinputlisting[linewidth=8cm]{./user_study/P5/input2.java}
    \label{fig:p1:i1}
    \end{subfigure}
    
    \begin{subfigure}[p]{\linewidth}
    \lstset{style=mystyle, xleftmargin=.0\textwidth, xrightmargin=0.\textwidth, linewidth=0.0\linewidth}
    \lstinputlisting[linewidth=8cm]{./examples/GCD/GCD_theirs.java}
    \label{fig:p1:ours}
    \end{subfigure}
    
  \caption{Precondition 5, Input 2, Group B.}
  \label{fig:P2}
\end{figure}
\begin{figure}
    \begin{subfigure}{\linewidth}
    \centering
    \lstset{style=mystyle, xleftmargin=.0\textwidth, xrightmargin=0.\textwidth, linewidth=0.0\linewidth}
    \lstinputlisting[linewidth=8cm]{./user_study/P5/input3.java}
    \label{fig:p1:i1}
    \end{subfigure}
    
    \begin{subfigure}[p]{\linewidth}
    \lstset{style=mystyle, xleftmargin=.0\textwidth, xrightmargin=0.\textwidth, linewidth=0.0\linewidth}
    \lstinputlisting[linewidth=8cm]{./examples/GCD/GCD_theirs.java}
    \label{fig:p1:ours}
    \end{subfigure}
    
  \caption{Precondition 5, Input 3, Group B.}
  \label{fig:P2}
\end{figure}
